# Supplementary material for: Argus: Interactive a priori Power Analysis
Source: arXiv:2009.07564 source file (2020-09-16)
Supplement: Supplementary file 1 [file S1-Argus-Appendices.pdf]

# Argus: Interactive *a priori* Power Analysis (Appendices)

Xiaoyi Wang, Alexander Eiselmayer, Wendy E. Mackay, Kasper Hornbæk, Chat Wacharamanotham

## Appendix A Differences in Standardized Effect Sizes Formulation

For a **between-subjects design**, we first calculate mean ($M_1$, $M_2$) and standard deviation ($s_1$, $s_2$) for each group. The simple effect size is the difference between the means, and the standardizer is an average of the standard deviations weighed by the sample size of each group ($N_x$).

$$d = \frac{M_2 - M_1}{s_p}, \qquad s_p = \sqrt{\frac{(N_1-1)s_1^2 + (N_2-1)s_2^2}{N_1+N_2-2}}$$

Suppose, however, that we **block by handedness** i.e. separating participants into left- and right-handed before randomly assigning each group to the two conditions. The standardizer requires scaling $s_p$ with a factor that excludes the between-block variance $s_b$:

$$d = \frac{M_2 - M_1}{s_p\sqrt{1 - s_b^2/s_p^2}}, \qquad s_b^2 = N_{LH}(M_{LH} - M_{all}) + N_{RH}(M_{RH} - M_{all})$$

For a **within-subjects design**, the change happens at the simple effect size. The differences between the two conditions are calculated individually for each participant before being averaged to be the simple effect size ($M_{diff}$). The standardizer ($s_{av}$) is the average of the standard deviation of the two conditions.

$$d = \frac{M_{diff}}{s_{av}}, \qquad s_{av} = \sqrt{\frac{s_1^2 + s_2^2}{2}}$$

## Appendix B Propagation Algorithm

**procedure** PropagateChange(nodes $n$, difference $d$)
 $C \leftarrow$ ChildrenOf($n$)
 $C_u \leftarrow$ UnlockedNodes($C$)
 **for** $c \in C_u$ **do** ▷ Top-down propagation
  $c \leftarrow d \times \|C\| / \|C_u\|$
 **end for**
 Update(n)
**end procedure**
**procedure** Update(node $n$)
 $v_{past} \leftarrow n.value$
 $C \leftarrow$ ChildrenOf($n$)
 $n.value \leftarrow (\sum_{c \in C} c.value) / \|C\|$
 $p \leftarrow$ ParentOf($n$)
 **if** IsUnlocked($p$) **then**
  Update($p$) ▷ Bottom-up update
 **else** ▷ If the parent is locked, . . .
  $d \leftarrow n.value - v_{past}$
  **for** $s \in$ Siblings($n$) **do** ▷ . . . distribute to siblings
   PropagateChange($s$, $-d$)
  **end for**
 **end if**
**end procedure**


- *Xiaoyi Wang and Kasper Hornbæk are with the University of Copenhagen, Denmark. E-Mail: {xiaoyi.wang, kash}@diku.dk.*
- *Alexander Eiselmayer and Chat Wacharamanotham are with the University of Zurich, Switzerland. E-Mail: {eiselmayer, chat}@ifi.uzh.ch.*
- *Wendy E. Mackay is with Univ. Paris-Sud, CNRS, Inria, Université Paris-Saclay, France. E-Mail: mackay@lri.fr.*


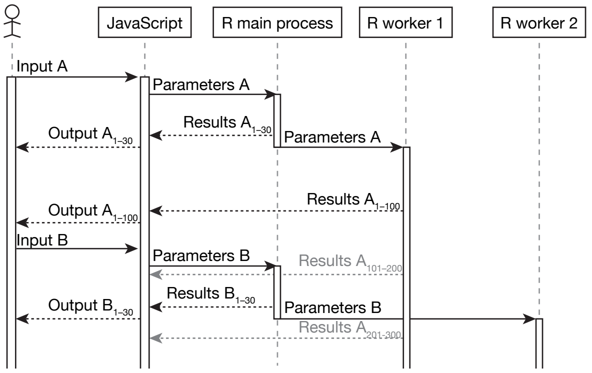


Fig. 1: A sequence diagram shows how *Argus* progressively receives and displays simulation results for a responsive user interface. Grey lines represent the results that are not shown on screen but stored for use when the user navigates back through the history.

## Appendix C Computation Architecture

Typical Shiny applications depend upon a reactive programming model: A change of an input control in the web browser is sent to R for calculation, and the results are returned to update the visualization. However, each user interaction in *Argus* can potentially trigger a time-consuming computation that could render the user interface unresponsive. *Argus* thus only uses Shiny to provide direct communication between R and JavaScript [1]. R returns computational results to JavaScript asynchronously, which ensures that the interface remains responsive. Fig. 1 shows a sample scenario: After receiving input A, the simulator computes a preview (Results $A_{1-30}$) and sends it back to JavaScript to be visualized. Subsequent results are sent back to JavaScript until the computation is complete. Suppose the user triggers Input B while the previous simulation is still running. *Argus* calculates the preview results ($B_{1-30}$) and pushes the updates to the user interface. Remaining calculations of parameter set A are calculated in parallel on a separate worker process and gradually sent back to the JavaScript side for storage. When the user revisits an earlier history point, previously stored output immediately shows results without requiring additional computation, which makes the history view fully responsive.

## Appendix D Think-aloud Study

To validate *Argus*, we conducted an observational study that captures participants' exploration process and insights on power analysis. We focused on the following research question: what insights can researchers gain from being able to interactively explore the impact of design choices (e.g., number of replication, number of participants, counterbalancing) for their experiments.

### D.1 Method

We used a think-aloud protocol where participants voice their observations and reasoning [5], and then performed a qualitative analysis of the results with affinity diagramming. Our analysis focused on *insights* that participants gained [6]. The study design and the analysis plan are preregistered at [click here for an anonymized URL on osf.io], and were conducted as such—unless stated otherwise below.

Table 1: Background information of the participants.

| | Expertise | Academic Level | Country | | |
|---|---|---|---|---|---|
| $P1_E$ | Experienced | Senior Scientist | FR | Lab1 | |
| $P2_E$ | Experienced | Senior Scientist | FR | Lab1 | |
| $P3_N$ | Novice | Ph.D. Student | FR | Lab1 | |
| $P4_E$ | Experienced | Post-doc | DK | Lab2 | (remote) |
| $P5_E$ | Experienced | Ph.D. Student | DE | Lab3 | (remote) |
| $P6_N$ | Novice | Ph.D. Student | DK | Lab2 | (remote) |
| $P7_N$ | Novice | Ph.D. Student | DK | Lab2 | (remote) |
| $P8_N$ | Novice | Ph.D. Student | CH | Lab4 | |
| $P9_N$ | Novice | Post-doc | FR | Lab1 | (remote) |

#### D.1.1 Participants

We recruited nine male participants from four different research labs, in four different countries, including junior (Ph.D. candidates) and senior researchers. Note that the types of insights that each participant might gain from using *Argus* depends on their prior experience with experiment design and *a priori* power analysis, and may not correlate directly with their academic level. However, researchers trained by the same institution may share the same experiment design philosophy. We interviewed each participant about their prior experience with planning, conducting, and analyzing experiment data, and classified them as novice ($P_{iN}$) or experienced ($P_{iE}$). For the latter group, researchers have several years of experience with controlled experiments in the field of HCI and/or VIS. Three participants (2 experienced, 1 novice) participated locally and the rest participated remotely. Each participant received the equivalent of a 30 EUR gift card.

#### D.1.2 Apparatus

We used an earlier version of Argus that did not include the whole-experiment practice effect in the *Confound* sliders. Local participants used *Argus* installed on a Macbook Pro (15-inch, 2.5GHz, MacOS 10.14), with QuickTime to record their screens. Remote participants accessed *Argus* via Shinyapps.io, with Skype for their interviews and screen recordings.

#### D.1.3 Procedure

**Training:** After the participants gave an informed consent, they watched a video provided in the supplemental material. The video provides a short refresher on experiment design and statistics and gives an overview of *Argus*. During the video, two prompts encourage participants to pause and try out interactions with *Argus*. Participants can then freely try adjusting the parameters in a dummy experiment setting. Participants are encouraged to ask questions or seek clarifications. Prior to the task, we asked participants to ensure that they were able to use and felt comfortable using *Argus*.

**Testing:** The participants were asked to determine the sample size for a Fitts's law experiment similar to Douglas et al. [3]. The experiment compares two devices (a touchpad and a joystick) at three indices of difficulties (3, 5, and 7). To simulate prior domain knowledge for estimating effect sizes, each participant received an information package (pp. 7–11 of the preregistration) printed on paper:

1. A summary of Douglas et al.'s study with the overall means and SD of the movement time for each device. To simulate the prior knowledge about confounding variables, we also indicate that there was a mild learning effect. To simulate constraints in experiment planning, the description indicated that participants were tired at the end of the original experiment.
2. Excerpts from a trial table, with three Latin-square counterbalancing strategies: (1) Douglas et al.'s original design: blocked by the device variable; (2) blocked by the device variable and serial-order where all trials with the same device are performed back-to-back; and (3) serial-order by device without blocking.

Before starting to use *Argus*, participants can ask questions about these materials, but may not ask questions during the session.

The main task is to explore the parameters and find a realistic sample size given the resource constraints typical of experiments they have previously conducted. We also ask them to propose two other variants of the experiment design that would reduce the overall number of trials, given the participant fatigue indicated in the information package. We regularly remind participants to verbally describe their actions and to 'think aloud'.

**Post-task questionnaire and interview:** Participants rate their experience and the insights they gained during the study on a 5-point Likert-style questionnaire. We then interview them about the process and probed for further insights they gained about power analysis.

#### D.1.4 Data Collection and analysis

We video-recorded the screen, logged the interaction steps, recorded audio, and took field notes. Two of the co-authors used the field notes to guide a partial transcription for points that the participants voiced, including observations and insights. The transcriptions were coded with a top-down coding scheme based on the typology of data models [2]. Three of the co-authors performed a bottom-up thematic analysis together using the affinity diagram method [4].

In addition to the preregistered analysis, we also extract how the users move from clicking on one input control to another and calculated first-order transition probabilities. Although the transition probabilities did not capture how the users attend to views that does not require clicking—e.g., *Pairwise-difference* view and *Power Trade-off* view—they can indicate how the users explore the parameter space.

### D.2 Results

This section describes our observations of the participants' interactions with *Argus* and the insights they, and we gained. We will use "users" to refer to the participants in our study to avoid confusion with the "number of participants" term in *Argus*.

Overall, the majority of the users reported that they have gained new insights about experiment design (Fig. 2):"*the preview is very useful to understand the confound effects.*"($P9_N$). $P7_N$, $P8_N$ were not familiar with carry-over effect and practice effect but they expressed their understanding of the difference between these effects when they saw the previews. Five users applied their experience in conducting experiment to consider potential confounds. For example, $P8_N$ said *"adding more replications can yield higher power but participants may be tired [so] I need to increase the fatigue."* after increased the number of replications.

#### D.2.1 Causal inference about parameter relationships

Based on the interview and screen recording video, we coded users' expression of causality (e.g., changing X affect Y) between power analysis parameters. The results is shown in Table 2. The most frequent insights connect the number of replications and the number of participants to the power (Table 2 row A and B): *"The power is very high now. I am going to tweak replications and participants to see how power is going to change [...] reduce the number of participants, power drops down. It makes sense"* ($P4_E$). Participants also interpret the characteristics of the curve in *Power Trade-off* view: *"The power get stabled after a certain number of participants. The current number of participant is a bit too much. We can reduce the number"* ($P5_E$). These results are within our expectation because the *Power Trade-off* view directly shows this relationship.

According to the transition probabilities, the users switches between manipulating the group-means and the grand-mean during their exploration (Fig. 3, A). This result demonstrates the usefulness of these controls on top of the normal bar charts. The causal link between the expected mean to power and to the confidence intervals in the *Pairwise-difference* view were expressed by two users each (Table 2 row C and F). For example, $P1_E$ said *"now I am going to reduce power [. . . ] a lot"* after dragging two group-means close to each other.

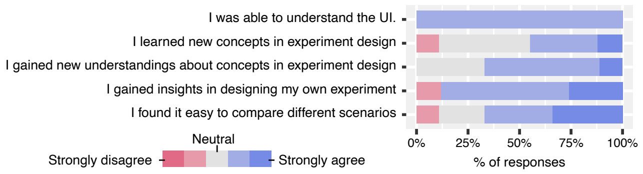


Fig. 2: Result of Study Questionnaire.

Table 2: Causality insights that the participants made, based on the coding of the interview data and screen recording video

| | From | To | Count | Participants |
|---|---|---|---|---|
| A | # replications | power | 6 | $P3_N$, $P5_E$, $P6_N$, $P7_N$, $P8_N$, $P9_N$ |
| B | # participants | power | 5 | $P1_E$, $P3_N$, $P4_E$, $P8_N$, $P9_N$ |
| C | expected means | power | 2 | $P1_E$, $P2_E$ |
| D | fatigue effect | power | 2 | $P7_N$, $P9_N$ |
| E | experiment design | power | 2 | $P4_E$, $P8_N$ |
| F | expected means | conf. interval | 2 | $P2_E$, $P5_E$ |
| G | experiment design | fatigue effect | 2 | $P3_N$, $P5_E$ |
| H | # replications | fatigue effect | 1 | $P6_N$ |
| I | practice effect | power | 1 | $P8_N$ |

The confound sliders had frequent transitions among themselves (Fig. 3, B), indicating that confounding effects were explored iteratively together by the users. Even though the carry-over effect was not mentioned on the information sheet, $P9_N$ felt it was necessary to consider it because "*there should be some [carry-over] effect between the first condition and the rests.*"

The exceptionally high transition probability from the practice effect slider to itself indicates that the users were more engaged in this effect more than others. This is opposite to Table 2 (row I) that only $P8_N$ links the practice effect to the power causally. We re-watch the interaction videos and found the reason of this contradiction. The users adjusts the confound sliders with an expectation to see the practice effect's influence. However, because of the initial value of the counterbalancing design (Latin Square & no serialization as used by [3]) and the number of replications (1 replication) does not allow the practice effect to manifest. In summary, the results suggests that when the causal link between the parameter and the power is moderated by the choices of the experiment design parameters, it could be more difficult for the users to make a set of parameters that can demonstrate the connection.

### D.2.2 The use of the *History* view

Five users tweaked expected confounds and observe how the power of adjacent nodes in the *History* view gradually changes. Four users repeatedly used the hover function to preview the difference. Two expert users use the branching to explore multiple strands of parameter configurations. These behaviors show that the *History* view successfully facilitates the exploration of statistical power.

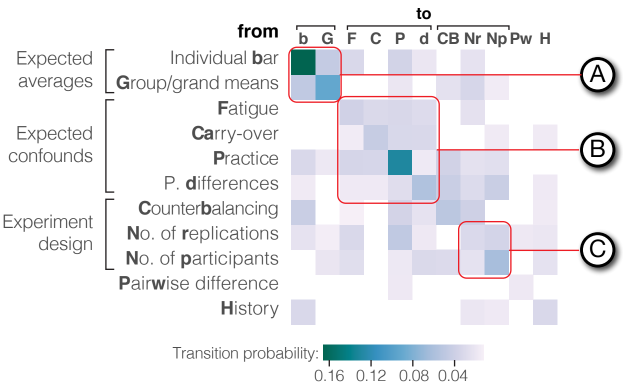


Fig. 3: Average transition probabilities among the input controls, averaged across participants. Three groups of controls (A–C) tends to be more frequently used together than others.

## References


[1] J. Cheng. Communicating with shiny via javascript. **https://shiny.rstudio.com/articles/communicating-with-js.html**, May 2018.

[2] I. K. Choi, T. Childers, N. K. Raveendranath, S. Mishra, K. Harris, and K. Reda. Concept-driven visual analytics: An exploratory study of model- and hypothesis-based reasoning with visualizations. In *Proceedings of the 2019 CHI Conference on Human Factors in Computing Systems*, CHI '19, pp. 68:1–68:14. ACM, New York, NY, USA, 2019. doi: 10.1145/3290605.3300298

[3] S. A. Douglas, A. E. Kirkpatrick, and I. S. MacKenzie. Testing pointing device performance and user assessment with the iso 9241, part 9 standard. In *Proceedings of the SIGCHI Conference on Human Factors in Computing Systems*, CHI '99, pp. 215–222. Association for Computing Machinery, New York, NY, USA, 1999. doi: 10.1145/302979.303042

[4] K. Holtzblatt and H. Beyer. *Contextual design: Design for life*. Morgan Kaufmann, 2016.

[5] C. Lewis. Using the "thinking-aloud" method in cognitive interface design. Research Report RC 9265 (#40713), IBM Thomas J. Watson Research Center, Yorktown Heights, NY, February 1982.

[6] P. Saraiya, C. North, and K. Duca. An insight-based methodology for evaluating bioinformatics visualizations. *IEEE Transactions on Visualization and Computer Graphics*, 11(4):443–456, 2005.
